# Supplementary material for: Plasmon-Enabled High-Precision Single Molecule Localization Microscopy over an Extended Field of View
Source: arXiv:2606.31758 source file (2026-11-30)
Supplement: Supplementary file 1 [file supplementary.tex]

\documentclass[pra, aps, twocolumn, %groupedaddress, %showpacs, 
superscriptaddress]{revtex4-2}

\usepackage{slashed}
\usepackage{graphicx}
\usepackage{comment}
\usepackage[usenames, dvipsnames]{color}
\usepackage{graphics}
\usepackage{hyperref}
\usepackage{appendix}
%\titlespacing{\section}{0pt}{0pt}{0pt}
%\usepackage{graphicx,subcaption}
\usepackage{bm}
\usepackage{amsfonts}
\usepackage{amsmath}
\usepackage{soul}

\hypersetup{
colorlinks=true,
urlcolor=blue,
linkcolor=blue,
linktoc=page,
citecolor=blue}

% \everymath{\displaystyle}  
\begin{document}

\title{Supplemental Material for Plasmon-Enabled High-Precision Single Molecule Localization Microscopy over an Extended Field of View}

\author{Muzzamal I. Shaukat}
\thanks{These authors contributed equally to this work.}
\affiliation{Institute for Quantum Science and Engineering}
% \email{..........}
\author{Carlos E. Rodriguez}
\thanks{These authors contributed equally to this work.}
\affiliation{Department of Physics and Astronomy\\
Texas A\&M University, College Station, Texas 77843, USA}
% \email{..........}
\author{M. Suhail Zubairy}
\email{zubairy@tamu.edu}
\affiliation{Institute for Quantum Science and Engineering}
\affiliation{Department of Physics and Astronomy\\
Texas A\&M University, College Station, Texas 77843, USA}
\author{Oumeng Zhang}
\email{ozhang@tamu.edu}
\affiliation{Institute for Quantum Science and Engineering}
\affiliation{Department of Physics and Astronomy\\
Texas A\&M University, College Station, Texas 77843, USA}
%\pacs{71.36.+c 03.75.Lm 14.80.Hv}
%\pacs{67.85.Hj 42.50.Lc 42.50.-p 42.50.Md 03.67.Bg}

\maketitle

\section{
Water-clad MDM dispersion with experimentally determined permittivity}

We consider a finite-thickness plasmonic structure consisting of a dielectric spacer of thickness \(t_d\) and permittivity \(\varepsilon_d\), confined between two identical metal films of thickness \(t_m\) and complex frequency-dependent permittivity \(\varepsilon_m(\omega)\), embedded in an external dielectric medium of permittivity \(\varepsilon_w\). The resulting multilayer geometry is
$
\mathrm{w}\,|\,\mathrm{m}(t_m)\,|\,\mathrm{d}(t_d)\,|\,\mathrm{m}(t_m)\,|\,\mathrm{w}$. Because the structure is translationally invariant along the propagation direction, the guided plasmonic modes propagate with a complex longitudinal wavevector \(\beta\). For transverse-magnetic (TM) polarization, Maxwell's equations in each homogeneous region yield evanescent field solutions characterized by transverse decay constants $
\kappa_j
=
\left(\beta^2-k_0^2\varepsilon_j\right)^{1/2}$,
where \(j\in\{w,m,d\}\) and $
k_0=\omega/c$. 
The finite metal claddings together with the external dielectric medium can be incorporated through a reduced admittance \cite{economou_surface_1969,burke_surface-polariton-like_1986},
%Solving Maxwell's equations subject to the TM boundary conditions at the metal--dielectric interfaces yields an effective reduced admittance describing the finite metal claddings and the external dielectric medium,
%Following the standard multilayer transfer-matrix formalism \cite{Abeles1950,burke_surface-polariton-like_1986,Berini2009}, the finite metal claddings together with the external dielectric medium can be represented through an effective reduced admittance
\begin{eqnarray}
P_{\mathrm{in}}^{(m)}
&=&
P_m
\frac{
P_w+P_m\tanh(\kappa_m t_m)
}{
P_m+P_w\tanh(\kappa_m t_m)
}
\end{eqnarray}
with
$P_j=\kappa_j/\varepsilon_j$.
The symmetry of the structure allows the guided gap-plasmon modes to be classified according to their parity. For the even magnetic-field branch, corresponding to the long-range gap-plasmon mode, the dispersion relation becomes
\begin{equation}
\frac{\kappa_d}{\varepsilon_d}
\tanh\left(
\frac{\kappa_d t_d}{2}
\right)
+
P_{\mathrm{in}}^{(m)}
=
0.
\label{eqn:FiniteMDMDispersion}
\end{equation}
The corresponding odd-parity branch is obtained by replacing the hyperbolic tangent by a hyperbolic cotangent. 
The dielectric response of the metallic layers is described using the experimentally measured optical constants of Johnson and Christy \cite{johnson_optical_1972}, from which the complex refractive index $\tilde n=n+ik$ is obtained. The metal permittivity then follows as $ \varepsilon_m = \tilde n^{\,2} = \varepsilon_m' + i\varepsilon_m''$, with $\varepsilon_m'=n^2-k^2$ and $\varepsilon_m''=2nk$. Because the metal permittivity is complex, the propagation constant is likewise complex, $\beta=\beta'+i\beta''$. The real and imaginary parts of $\beta$ are obtained by numerically solving Eq.~(\ref{eqn:FiniteMDMDispersion}) at each frequency. In the limit $t_m\rightarrow\infty$, the effective admittance approaches $ P_{\mathrm{in}}^{(m)} \rightarrow \kappa_m/\varepsilon_m$, and Eq.~(\ref{eqn:FiniteMDMDispersion}) reduces to the familiar metal--dielectric--metal gap-plasmon dispersion relation. As an illustration, Table~\ref{tab:beta_values} lists representative values of the complex propagation constant
\(\beta=\beta'+i\beta''\)
for the finite water-clad metal--dielectric--metal structure studied here, with \(\varepsilon_d=2.25\). The large values of $\beta'$ reflect strong subwavelength confinement, while the finite value of $\beta''$ determines the propagation length and ultimately limits the attainable resolution enhancement.

\begin{table}[ht!]
  \caption{Representative values of the complex propagation constant
$\beta=\beta'+i\beta''$
for the even TM gap-plasmon mode supported by the finite
water--metal--dielectric--metal--water structure. The outer water cladding has permittivity
$\varepsilon_w=1.77$,
the dielectric spacer has permittivity
$\varepsilon_d=2.25$
and the free-space wavenumber is
$k_0=2\pi/\lambda$.}
  \label{tab:beta_values}
  \begin{ruledtabular}
  \begin{tabular}{ccccc}
    $E$(eV) & $\beta'$(m$^{-1}$) & $\beta''$(m$^{-1}$) & $t_d$(nm) & $t_m$(nm)  \\
    \hline
    1.02  & $ 2.13 \times 10^7$ & $1.64\times 10^{5}$ & 10 & 20\\
    2.01  & $1.00 \times 10^8$ & $2.07\times 10^{6}$ & 3 & 20 \\
    2.01  & $6.34 \times 10^7$ & $1.00\times 10^{6}$ & 6 & 20 \\
    2.01  & $ 4.82 \times 10^7$ & $6.63\times 10^{5}$ & 10 & 20 \\
    2.01  & $ 3.04 \times 10^7$ & $3.44\times 10^{5}$ & 30 & 20 \\
    2.01  & $4.43 \times 10^7$ & $5.69\times 10^{5}$ & 10 & 30 \\
    2.01  & $4.26 \times 10^7$ & $5.19\times 10^{5}$ & 10 & 100 \\
    2.50  & $ 6.90 \times 10^7$ & $1.27\times 10^{6}$ & 10 & 20 \\
  \end{tabular}
  \end{ruledtabular}
\end{table}

\section{Cram\'er-Rao bound for localization}

To benchmark the performance of PIFLUX and compare it with other techniques, we compute the Cram\'er-Rao bound (CRB) from the Fisher information (FI) \cite{moon2000mathematical,chao_fisher_2016}.
The emission point-spread function (PSF) is modeled using a scalar Fourier-optics description,
\begin{equation}
\label{eqn:psf}
\text{PSF}(x,y)=A\left|\mathcal{F}\left\{\text{Circ}\left(\frac{n\rho}{\text{NA}}\right)\frac{\exp\!\left[i k_\text{em}(x u+y v)\right]}{\left(1-\rho^2\right)^{1/4}}\right\}\right|^2,
\end{equation}
where $\mathcal{F}$ denotes a 2D Fourier transform, $(u,v)$ are pupil-plane coordinates, $\rho=\sqrt{u^2+v^2}$, and $k_\text{em}=2\pi/\lambda_{\mathrm{em}}$. 
$\mathrm{Circ}(\cdot)$ is the circular pupil function set by the objective NA (with cutoff $\rho\le \mathrm{NA}/n$), and $A$ is a normalization factor chosen such that the PSF integrates to unity.

For an SM at position $(x,y)$ with total signal $s$ and total background $b$ per pixel (both summed over $N$ frames: $N=6$ for PIFLUX and SIMFLUX, $N=4$ for MINFLUX, and $N=1$ for conventional SMLM), we generated synthetic data under an independent Poisson noise model. Specifically, for frame $m$ the detected image is sampled as
\begin{equation}
I_{\mathrm{em},m}(x,y)\sim \mathrm{Poisson}\!\left(s\, I_{\mathrm{ex},m}(x,y)\,\mathrm{PSF}(x,y) + b/N\right),
\label{eqn:noiseModel}
\end{equation}
where $I_{\mathrm{ex},m}(x,y)$ is the excitation intensity profile for frame $m$, normalized such that $\sum_{m=1}^{N} I_{\mathrm{ex},m}(x,y)=1$.
The FI matrix for $(x,y)$ is then
\begin{align}
\mathrm{FI}&=\nonumber\\
&\sum_{m=1}^{N}\sum_{p}\frac{1}{I_{p,m}}
\begin{bmatrix}
\left(\partial_x I_{p,m}\right)^2 & \left(\partial_x I_{p,m}\right)\left(\partial_y I_{p,m}\right)\\
\left(\partial_x I_{p,m}\right)\left(\partial_y I_{p,m}\right) & \left(\partial_y I_{p,m}\right)^2
\end{bmatrix},
\end{align}
where $I_{m,p}$ is the expected photon count in pixel $p$ of frame $m$, and $\partial_x$ and $\partial_y$ denote derivatives with respect to the emitter position. The CRB is then given by the inverse Fisher information, $\text{CRB}=\text{FI}^{-1}$.

\begin{figure}[ht!]
    \centering
    \includegraphics[width=\linewidth]{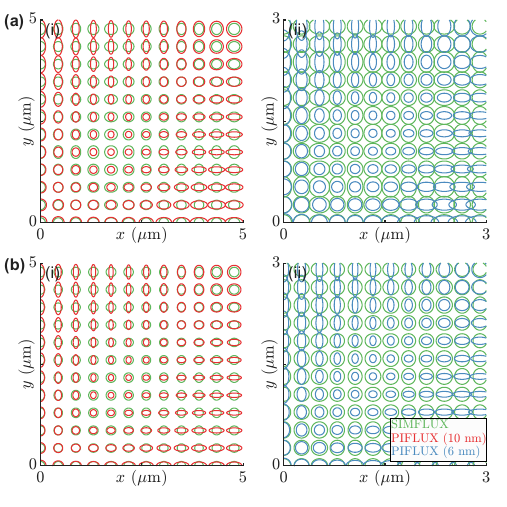}
    \caption{CRB covariance ellipses for lateral localization with 500 signal photons and total background levels of (a) 1 and (b) 20 photons per $(65~\mathrm{nm})^2$ pixel (summed over all six frames). PIFLUX with (i) $t_d=10$~nm and (ii) $t_d=6$~nm is compared with SIMFLUX. The ellipses are magnified by factors of 50 in (a) and 25 in (b) for visualization.}
    \label{fig:CRB_2D}
\end{figure}

We visualize the CRB comparison between PIFLUX (with $t_d=6$~nm and $t_d=10$~nm at 2.01~eV) and SIMFLUX (Fig.~\ref{fig:CRB_2D}). We plot CRB covariance ellipses to capture not only the one-dimensional precisions $\sigma_x^{(\mathrm{CRB})}$ and $\sigma_y^{(\mathrm{CRB})}$, but also the $x$--$y$ covariance. Across most of the field of view (5~\textmu m$\times$ 5~\textmu m for $t_d=10$~nm and 3~\textmu m$\times$ 3~\textmu m for $t_d=6$~nm), the PIFLUX ellipses are smaller than those of SIMFLUX for both high (Fig.~\ref{fig:CRB_2D}a) and low (Fig.~\ref{fig:CRB_2D}b) SBRs, indicating improved localization precision.

\begin{figure}[b!]
    \centering
    \includegraphics[width=\linewidth]{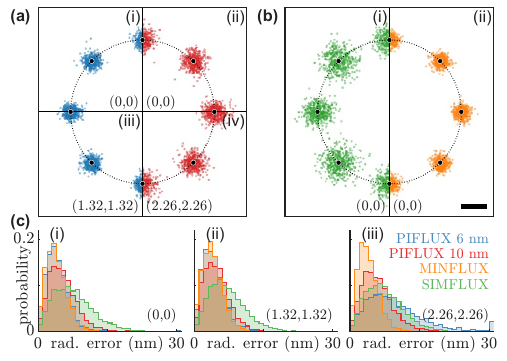}
    \caption{The localization estimates are shown against the ground-truth ring of a simulated NPC, with a total signal of 500 photons and a total background of 20 photons per pixel distributed across all frames (six for PIFLUX and SIMFLUX, four for MINFLUX). (a) PIFLUX: (i) $t_d=6$~nm and (ii) $t_d=10$~nm with the ring centered at the origin, and (iii) $t_d=6$~nm and (iv) $t_d=10$~nm with the ring at their optimal distances of $(1.32,1.32)$ and $(2.26,2.26)$~\textmu{}m, respectively. (b) Corresponding results for (i) SIMFLUX and (ii) MINFLUX. Scale bar: 20~nm.}
    \label{fig:FLUX20}
\end{figure}

\section{Maximum likelihood estimator}

Here, we present the details of the maximum-likelihood estimator. 
PIFLUX and SIMFLUX share the same phase-shifted acquisition and estimator, differing only in the illumination pattern, whereas MINFLUX was simulated with its standard donut-scanning scheme; all three localizations were obtained under the Poisson noise model of Eq. \ref{eqn:noiseModel}.
For PIFLUX, each phase shift of the excitation pattern generated an image using the scalar PSF (Eq. \ref{eqn:psf}) and the local excitation intensity (Eq. 1 of the main text). This resulted in three images per axis ($\varphi=0$, $2\pi/3$, and $4\pi/3$) and six in total.
Localization then proceeded in three stages across both axes. First, all six images were summed into a high signal-to-noise composite, then cross-correlated with a PSF template to bound an initial $5\times5$-pixel region of interest, balancing estimator performance against computational cost. A maximum-likelihood evaluation over a 500-point grid was next performed per axis within the region of interest to determine a coarse localization. Finally, the grid was refined around the coarse-stage maximum and its two neighboring grid points to yield the fine per-axis localizations, which were combined into the overall 2-D localization.

The NPC localization results under the low-SBR condition, complementing the high-SBR case of the main text, is presented in Fig~\ref{fig:FLUX20}. The simulation follows the same protocol, with the total background increased to 20 photons per pixel while the signal is kept at 500 photons. The localization accuracy and precision as functions of molecular position, for both high- and low-SBR conditions, are shown in Fig.~\ref{fig:ERR20}.

\begin{figure}[ht!]
    \centering
    \includegraphics[width=\linewidth]{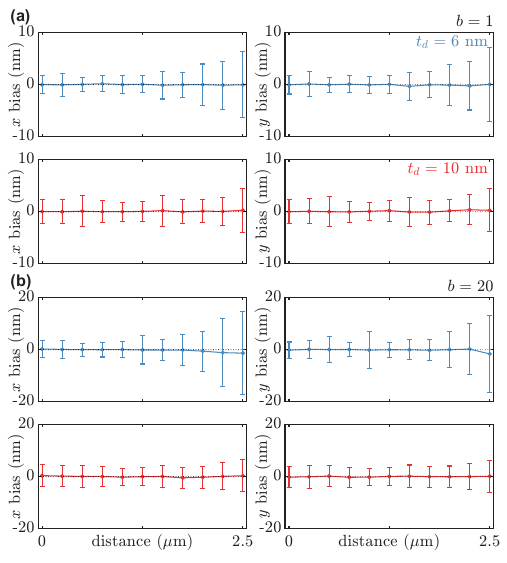}
    \caption{ Mean localization bias along $x$ and $y$ for emitters at varying diagonal distances from the origin, for (a) a background photon per pixel count of 1 and (b) a background photon per pixel count of 20. Error bars denote the standard deviation. The blue graphs represent $t_d=6$~nm PIFLUX while the red graphs represent $t_d=10$~nm PIFLUX.}
    \label{fig:ERR20}
\end{figure}

\vspace{0.1cm}

\section{Field-of-view limit set by the modulation envelope}

Fig.~\ref{fig:fov} further illustrates that the usable FOV in PIFLUX is set by the depth of the normalized minima within each period of the excitation pattern, and thus by the decay rate of the plasmonic modulation envelope, with FOV length inversely proportional to $\beta''$. As long as the valley within each period remains sufficiently low, the excitation retains strong sinusoidal modulation and the relative excitation intensities provide strong positional information for localization refinement. However, when the valley rises to approximately one-third of the peak intensity, the modulation contrast is noticeably reduced (Fig.~\ref{fig:fov}a), and the excitation pattern is better regarded as a sinusoidal variation on top of a large constant offset. In this regime, the spatially varying component is no longer dominant, so the ability to refine emitter position from intensity differences degrades accordingly. Comparing Figs.~\ref{fig:fov}a and \ref{fig:fov}b, the $t_d=10$~nm and $t_d=6$~nm designs exhibit different decay behaviors, which determine how quickly this loss of modulation contrast occurs and therefore how long strong localization performance can be maintained.

\begin{figure}[ht!]
    \centering
    \includegraphics[width=\linewidth]{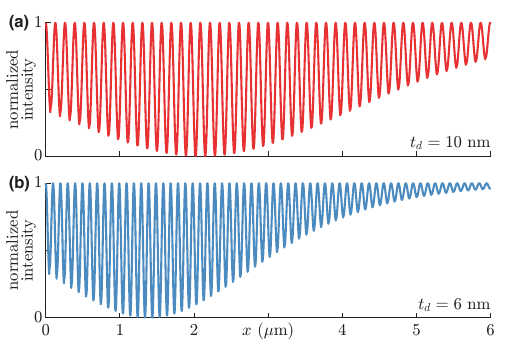}
    \caption{The FOV of PIFLUX is set by the normalized minima in each period of the excitation pattern. The patterns shown are computed at 2.01~eV ($\lambda_{\mathrm{ex}}=617$~nm) for (a) $t_d=10$~nm and (b) $t_d=6$~nm, and are normalized within each period (see Fig. 2 for normalization over the full pattern).}
    \label{fig:fov}
\end{figure}

\bibliography{references}

\onecolumngrid

\end{document}
